# Supplementary material for: CTI-HAL: A Human-Annotated Dataset for Cyber Threat Intelligence Analysis
Source: arXiv:2504.05866 source file (2025-04-08)
Supplement: Supplementary file 1 [file appendix.tex]

\appendix
\section*{Appendix}
\section{Documents}
This section of the appendix presents tables listing the documents used to create the dataset. Each table provides detailed information on the specific documents, with references to the analyzed APTs, offering a clear overview of the sources used during the annotation and analysis process.
\begin{table}[ht]
\begin{tabular}{|p{0.9\linewidth}|}
\hline
\multicolumn{1}{|c|}{\textbf{Title}}                                                              \\ \hline
Analysis of cyberattack on U.S. think tanks, non-profits, public sector by unidentified attackers \cite{microsoft_cyberattack_analysis}\\ \hline
COSMICDUKE Cosmu with a twist of MiniDuke \cite{fsecure_cosmicduke}                                                         \\ \hline
CrowdStrike’s work with the Democratic National Committee: Setting the record straight \cite{crowdstrike_dnc_intrusion}            \\ \hline
THE DUKES 7 YEARS OF RUSSIAN CYBERESPIONAGE \cite{fsecure_dukes_whitepaper}                                                       \\ \hline
“Forkmeiamfamous”: Seaduke, latest weapon in the Duke armory \cite{symantec_forkmeiamfamous}                                     \\ \hline
GRIZZLY STEPPE – Russian Malicious Cyber Activity \cite{cisa_grizzly_steppe}                                                \\ \hline
Not So Cozy: An Uncomfortable Examination of a Suspected APT29 Phishing Campaign \cite{google_not_so_cozy}                  \\ \hline
PowerDuke: Widespread Post-Election Spear Phishing Campaigns Targeting Think Tanks and NGOs \cite{volexity_powerduke}       \\ \hline
Unit 42 Technical Analysis: Seaduke \cite{unit42_seaduke_analysis}                                                               \\ \hline
The CozyDuke APT \cite{securelist_cozyduke}                                                                                \\ \hline
The MiniDuke Mystery: PDF 0-day Government Spy Assembler 0x29A Micro Backdoor \cite{kaspersky_miniduke}                     \\ \hline
Dissecting One of APT29's Fileless WMI and PowerShell Backdoors (POSHSPY) \cite{google_dissection_oneofap}                         \\ \hline
\end{tabular}
\caption{APT29 \cite{apt29_emulation_library}}
\label{tab:apt29_docs}
\end{table}

\begin{table}[ht]
\begin{tabular}{|p{0.9\linewidth}|}
\hline
\multicolumn{1}{|c|}{\textbf{Title}}                                          \\ \hline
An APT Blueprint: Gaining New Visibility into Financial Threats \cite{bitdefender_financial_threats}              \\ \hline
Alleged Mastermind Behind Carbanak Crime Gang Arrested \cite{threatpost_carbanak_mastermind}                        \\ \hline
Arrests Put New Focus on CARBON SPIDER Adversary Group \cite{crowdstrike_carbon_spider}                        \\ \hline
Operation Grand Mars: a comprehensive profile of Carbanak activity in 2016/17 \cite{trustwave_grand_mars} \\ \hline
The Great Bank Robbery: the Carbanak APT \cite{kaspersky_great_bank_robbery}                                      \\ \hline
CARBANAK APT THE GREAT BANK ROBBERY \cite{kaspersky_carbanak_apt_pdf}                                          \\ \hline
Behind the CARBANAK Backdoor \cite{google_carbanak_backdoor}                                                  \\ \hline
New Carbanak / Anunak Attack Methodology \cite{trustwave_carbanak_new_methodology}                                      \\ \hline
Carbanak Continues To Evolve: Quietly Creeping into Remote Hosts \cite{trustwave_carbanak_evolution}              \\ \hline
Carbanak Group uses Google for malware command-and-control \cite{forcepoint_carbanak_google_c2}                    \\ \hline
\end{tabular}
\caption{Carbanak \cite{carbanak_emulation_library}}
\label{tab:carbanak_docs}
\end{table}

\begin{table}[ht]
\begin{tabular}{|p{0.9\linewidth}|}
\hline
\multicolumn{1}{|c|}{\textbf{Title}}                                                                                                                          \\ \hline
FOLLOW THE MONEY: DISSECTING THE OPERATIONS OF THE CYBER CRIME GROUP FIN6 \cite{mandiant_fin6_report}                                                                                     \\ \hline
FIN6 Cybercrime Group Expands Threat to eCommerce Merchants \cite{visa_fin6_ecommerce}                                                                                                   \\ \hline
FIN6 group goes from compromising PoS systems to deploying ransomware \cite{cyware_fin6_pos_ransomware}                                                                                         \\ \hline
Navigating the MAZE: Tactics, Techniques and Procedures Associated With MAZE Ransomware Incidents \cite{google_maze_ransomware}                                                            \\ \hline
New Global Cyber Attack on Point of Sale Systems \cite{morphisec_fin6_pos_attack}                                                                                                              \\ \hline
ITG08 (aka FIN6) Partners With TrickBot Gang, Uses Anchor Framework \cite{securityintelligence_fin6_trickbot}                                                                                           \\ \hline
More\_eggs, Anyone? Threat Actor ITG08 Strikes Again \cite{securityintelligence_moreeggs}                                                                                                          \\ \hline
Pick-Six: Intercepting a FIN6 Intrusion, an Actor Recently Tied to Ryuk and LockerGoga Ransomware \cite{google_fin6_intrusion}                                                            \\ \hline
Another Victim Of The Magecart Assault Emerges: Newegg \cite{malwarenews_magecart_newegg}                                                                                                        \\ \hline
Inside the Breach of British Airways: How 22 Lines of Code Claimed 380,000 Victims. How We Used Machine Learning to to Pinpoint the Magecart Crime Syndicate. \cite{schoenbaum_british_airways_breach}  \\ \hline
Magecart Card Skimmers Injected Into Online Shops \cite{trendmicro_fin6_magecart}                                                                                                           \\ \hline
Fake Jobs: Campaigns Delivering More\_eggs Backdoor via Fake Job Offers \cite{proofpoint_moreeggs_fake_jobs}                                                                                       \\ \hline
\end{tabular}
\caption{FIN6 \cite{fin6_emulation_library}}
\label{tab:fin6_docs}
\end{table}

\begin{table}[ht]
\begin{tabular}{|p{0.9\linewidth}|}
\hline
\multicolumn{1}{|c|}{\textbf{Title}}                                        \\ \hline
Cyberthreats to financial institutions 2020: Overview and predictions \cite{securelist_financial_predictions_2020}                      \\ \hline
Mahalo FIN7: Responding to the Criminal Operators’ New Tools and Techniques \cite{google_mahalo_fin7}               \\ \hline
Deep Insight into “FIN7” Malware Chain: From Office Macro Malware to Lightweight JS Loader \cite{sentinelone_fin7} \\ \hline
FIN7.5: the infamous cybercrime rig “FIN7” continues its activities \cite{securelist_fin7}                        \\ \hline
FIN7 Revisited: Inside Astra Panel and SQLRat Malware \cite{flashpoint_fin7}                                     \\ \hline
Profile of an Adversary – FIN7 \cite{deepwatch_fin7}                                                             \\ \hline
FIN7 Not Finished – Morphisec Spots New Campaign \cite{morphisec_fin7_campaign}                                           \\ \hline
On the Hunt for FIN7: Pursuing an Enigmatic and Evasive Global Criminal Operation \cite{google_fin7_global_operation}          \\ \hline
HOW FIN7 ATTACKED AND STOLE DATA \cite{justice_fin7}                                                           \\ \hline
Footprints of Fin7: Pushing New Techniques to Evade Detection \cite{gigamon_fin7_evasion}                             \\ \hline
FIN7 Group Uses JavaScript and Stealer DLL Variant in New Attacks \cite{talos_fin7_stealer}                          \\ \hline
FIN7/Carbanak threat actor unleashes Bateleur JScript backdoor \cite{proofpoint_fin7_backdoor}                             \\ \hline
Footprints of FIN7: Tracking Actor Patterns (Part 2) \cite{gigamon_fin7_patterns_2}                                      \\ \hline
Footprints of Fin7: Tracking Actor Patterns (Part 1) \cite{gigamon_fin7_patterns_1}                                       \\ \hline
Behind the CARBANAK Backdoor \cite{fireeye_carbanak_backdoor}                                                              \\ \hline
FIN7 Takes Another Bite at the Restaurant Industry \cite{morphisec_fin7_restaurants}                                        \\ \hline
To SDB, Or Not To SDB: FIN7 Leveraging Shim Databases for Persistence \cite{google_fin7_shim_databases}                     \\ \hline
FIN7 Evolution and the Phishing LNK \cite{google_fin7_phishing}                                                        \\ \hline
\end{tabular}
\caption{FIN7 \cite{fin7_emulation_library}}
\label{tab:fin7_docs}
\end{table}

\begin{table}[ht]
\begin{tabular}{|p{0.9\linewidth}|}
\hline
\multicolumn{1}{|c|}{\textbf{Title}}                                                                            \\ \hline
APT34: The Helix Kitten Cybercriminal Group Loves to Meow Middle Eastern and International Organizations \cite{cyware_apt34}        \\ \hline
Threat Brief: Iranian-Linked Cyber Operations \cite{unit42_iran_ops}                                                                  \\ \hline
Please Confirm You Received Our APT \cite{fortinet_apt34}                                                                             \\ \hline
New Targeted Attack in the Middle East by APT34, a Suspected Iranian Threat Group, Using CVE-2017-11882 Exploit \cite{mandiant_apt34} \\ \hline
New Iranian Campaign Tailored to US Companies Utilizes an Updated Toolset \cite{intezer_iranian_campaign}                                       \\ \hline
IRAN’S APT34 RETURNS WITH AN UPDATED ARSENAL \cite{checkpoint_apt34}                                                                    \\ \hline
APT34 targets Jordan Government using new Saitama backdoor \cite{threatdown_apt34}                                                      \\ \hline
Behind the Scenes with OilRig \cite{unit42_oilrig}                                                                                   \\ \hline
\end{tabular}
\caption{OilRig \cite{oilrig_emulation_library}}
\label{tab:oilrig_docs}
\end{table}

\begin{table}[ht]
\centering
\begin{tabular}{|p{0.9\linewidth}|}
\hline
\multicolumn{1}{|c|}{\textbf{Title}} \\ \hline
Six Russian GRU Officers Charged in Connection with Worldwide Deployment of Destructive Malware and Other Disruptive Actions in Cyberspace \cite{justice_gru} \\ \hline
Carbon Black Threat Research Technical Analysis: Petya / NotPetya Ransomware \cite{vmware_petya} \\ \hline
CRASHOVERRIDE Analysis of the Threat to Electric Grid Operations \cite{dragos_crashoverride} \\ \hline
Mapping MITRE ATT\&CK to SandWorm APT’s Global Campaign \cite{reliaquest_sandworm} \\ \hline
ExPetr/Petya/NotPetya is a Wiper, Not Ransomware \cite{securelist_expetr} \\ \hline
Olympic Destroyer Takes Aim At Winter Olympics \cite{talos_olympicdestroyer} \\ \hline
Cyber-Attack Against Ukrainian Critical Infrastructure \cite{cisa_ics_alert} \\ \hline
Sandworm Team and the Ukrainian Power Authority Attacks \cite{google_sandworm} \\ \hline
\end{tabular}
\caption{Sandworm \cite{sandworm_emulation_library}}
\label{tab:sandworm_docs}
\end{table}

\begin{table}[ht]
\centering
\begin{tabular}{|p{0.9\linewidth}|}
\hline
\multicolumn{1}{|c|}{\textbf{Title}} \\ \hline
Trickbot Adds Credential-Grabbing Capabilities \cite{trendmicro_trickbot} \\ \hline
Big Game Hunting with Ryuk: Another Lucrative Targeted Ransomware \cite{crowdstrike_ryuk} \\ \hline
Ryuk wakes from hibernation; FBI, DHS warn of healthcare attacks \cite{cybersecuritydive_ryuk} \\ \hline
\end{tabular}
\caption{WizardSpider \cite{wizardspider_emulation_library}}
\label{tab:wizardspider_docs}
\end{table}
